# Supplementary material for: Hardware/Software Co-verification Using Path-based Symbolic Execution
Source: arXiv:2001.01324 source file (2020-01-05)
Supplement: Supplementary file 1 [file appendix.tex]

\section {Appendix}

\section {Netlist at different levels of abstractions}
%Figure~\ref{fig:v2c-example} shows the Verilog RTL 
%design described at different levels of granularity: \emph{bit-level},
%\emph{word-level}, \emph{software-level}. Note that the word-level 
%netlist shown here is not a standard representation but is tool specific. 
One of the challenges in the Verilog to C translation is the handling of 
parallelism, which arises from dependencies between procedural blocks 
and continuous (wire) assignments or combinatorial exchanges (feedback loop) 
between modules, as shown in Figure~\ref{fig:v2c-example}. 
The code on the left shows a Verilog design with a combinatorial 
feedback loop. The equivalent bit-level, word-level netlist and software netlist 
in C is shown in the second, third and forth column respectively.
The top level module $\mathit{top}$ in the Verilog code instantiates two sub-modules, $A$ and $B$. 
The combinatorial exchanges between module $\mathit{top}$, $A$ and $B$ are modeled in the 
function $A\_comb()$ in the software netlist model. The function $A\_comb()$ contains
an assumption that encodes the dependencies over corresponding signals in the 
combinatoral logic. The sequential clocked block in module $A$ is modeled in a separate 
function $A\_seq()$. The difference between word-level 
netlist and software netlist is that the control-flow 
structure is retained in the later. Whereas, the control-flow structure 
is lost in bit-level or word-level netlist. Thus, the translation 
to software netlist gives an opportunity for the backend analysis engine to 
exploit the feasibility of the control-flow structure using various 
path-based symbolic execution techniques, such as eager path-pruning, 
path-merging or loop acceleration techniques.  

\begin{figure}[h]
\tiny
\begin{tabular}{l|l|l|l}
\hline
 Verilog & Bit-level netlist & Word-level netlist & Software netlist \\
\hline
\begin{lstlisting}[mathescape=true,language=Verilog]
module A(clk,x,bar,
        foo,y,msg);
 input clk,x,bar;
 output y,foo,msg;
 reg [2:0] q;
 wire [2:0] msg; 
 assign foo=x;
 assign y=bar;
 assign msg = q;
 always @(posedge clk) 
 begin
  if(x) q = foo+1;
  else  q = y+5;  
 end
endmodule

module B(foo,bar);
input foo;
output bar;
assign bar=foo;
endmodule

module top(x,clk);
 input x, clk;
 wire x,y,foo,bar,clk;
 wire [2:0] msg;
 A a(.clk(clk), .x(x),
 .bar(bar),.foo(foo),
 .y(y), .msg(msg));
 B b(foo,bar);
endmodule
\end{lstlisting}
&
\begin{lstlisting}[mathescape=true,language=C]
Variable map:
  input[0]=9,input[1]=10, input[2]=11, 
  input[3]=12, input[4]=13, input[5]=14, 
  input[6]=15, input[7]=19, input[8]=23, 
  input[9]=24, input[10]=25, input[11]=38, 
  top.b.foo=8, top.a.bar=4, top.a.x=3, 
  top.a.clk=2, top.clk=1, top.x=0 
  
  Wire: top.b.bar=8,top.a.q_aux1[0]=!4,
  top.a.q_aux1[1]=4,top.a.q_aux1[2]=true,
  top.a.q_aux0[0]=!3,top.a.q_aux0[1]=3,
  top.a.q_aux0[2]=false,top.a.msg[0]=5, 
  top.a.msg[1]=6,top.a.msg[2]=7, 
  top.msg[0]=23,top.msg[1]=24,
  top.msg[2]=25,top.bar=38,top.foo=19,
  top.y=15,top.a.foo=3,top.a.y=4, 
  
  Latch: top.a.q[0]=5, 
  top.a.q[1]=6, top.a.q[2]=7

Next state functions:
  NEXT(top.a.q[0])=!var(3) & !var(4)
  NEXT(top.a.q[1])=!(!var(3) & 
  !(!var(3) & var(4)))
  NEXT(top.a.q[2])=!var(3)

Transition constraints: 
  !(var(4) & !var(15)) & !(!var(4) & var(15))
  !(var(3) & !var(19)) & !(!var(3) & var(19))
  !(var(5) & !var(23)) & !(!var(5) & var(23))
  !(var(6) & !var(24)) & !(!var(6) & var(24))
  !(var(7) & !var(25)) & !(!var(7) & var(25))
  !(var(8) & !var(38)) & !(!var(8) & var(38))
  !(var(2) & !var(1)) & !(!var(2) & var(1))
  !(var(3) & !var(0)) & !(!var(3) & var(0))
  !(var(4) & !var(38)) & !(!var(4) & var(38))
  !(var(8) & !var(19)) & !(!var(8) & var(19))
  TRUE
  \end{lstlisting}
&
\begin{lstlisting}[mathescape=true,language=C]
State constraints:
top.a.foo==top.a.x
top.a.y==top.a.bar
top.a.msg==top.a.q
top.a.q_aux0== 
top.a.foo+3'b1
top.a.q_aux1== 
top.a.y+3'b101
top.a.clk==top.clk
top.a.x==top.x
top.a.bar==top.bar
top.a.foo==top.foo
top.a.y==top.y
top.a.msg==top.msg
top.b.bar==top.b.foo
top.b.foo==top.foo
top.b.bar==top.bar

Transisition 
constraints:
next(top.a.q)==
top.a.x? 
top.a.q_aux0:
top.a.q_aux1
\end{lstlisting}
&
\begin{lstlisting}[mathescape=true,language=C]
typedef unsigned char _u8;
struct module_A {
 _Bool clk,x,bar,y,foo;
 _u8 q; }
struct module_B {
  _Bool foo, bar; };
struct module_top {
  _Bool x,y,foo,bar,clk;
  struct module_A a;
  struct module_B b; };
extern struct module_top top;

void A_seq() {
 if(top.x)
  top.a.q = top.a.foo + 1;
 else
  top.a.q = top.a.y + 5;
}

void A_comb() {
  assume((top.a.foo == top.a.x)
  && (top.a.y == top.a.bar) 
  && (top.a.x == top.x)
  && (top.a.foo == top.foo) 
  && (top.a.bar == top.bar)
  && (top.a.y == top.y) 
  && (top.b.bar == top.b.foo)
  && (top.b.foo == top.foo) 
  && (top.b.bar == top.bar)
  && (top.msg == top.a.msg) 
  && (top.a.q == top.a.msg));
}
void main() {
 A_seq(); 
 A_comb();
}
\end{lstlisting}
\\
\hline
\end{tabular}
\caption{Verilog design representation at different levels of granularity}
\label{fig:v2c-example}
\end{figure}

\section {Structure of Software netlist model}
\textbf{Software netlist Model:} The pseudo-code for the software netlist 
model generated by \emph{v2c} is shown in figure~\ref{figure:structure}.

\begin{figure}[t]
\tiny
\begin{tabular}{l}
\hline
 Pseudo-code for software-netlist model \\
\hline
\begin{lstlisting}[mathescape=true,language=C]
// parameter definition
// macro definition
struct state_elements_design
  // declare all state-holding elements
  // of the current module 
};
struct state_elements_design sdesign;
int initial_block() { //initialization of nets }
// Input are passed by value and output by reference
int design (data_type input, data_type *output) {

  // shadow variable declaration
  declare shadow variables for 
  non-blocking assignments to 
  the register elements  
  
  // continuous assignments
  Place all continuous statements which 
  are only dependant on input
 
  // always block 
  Place the always block respecting
  intra-modular dependencies
  // procedural statements are bit-precise

  // continuous assignments
  Place all continuous statements which 
  are updated by signals that are 
  driven from the always block

  // Module instantiations 
  Place all module instances 
  with proper mapping of 
  input and output ports

} // end of design module

int main() {
  // local varaibles 
  declare all local variables 
  which are passed to the design 
  initial_block(); // call to initial block
  // check if the design is sequential.
  // if so, then put a  while(1) wrapper
  while(1) {
   // nondeterministic assignments
   nondeterministically assign inputs values  
   // call the design
   design(input, &output);
  }
  // Assertions 
  Place the C assertions here 
} //end main 
\end{lstlisting}
\\
\hline
\end{tabular}
\caption{Skeleton of the software netlist model generated by \emph{v2c}}
\label{figure:structure}
\end{figure}

%%===============================================================================\
\para{Bit-precise code generation:}
%%===============================================================================\
\emph{v2c} generates a bit-precise software netlist model in~C.  The tool
automatically handles complex bit-level operators in Verilog like
bit-select or part-select operators from a vector, concatenation operators,
reduction OR and other operators.  \emph{v2c} retains the word-level structure 
of the Verilog RTL and generates vectored expressions. 
Figure~\ref{figure:bit} shows Verilog code (at the top) and the generated C
expressions (at the bottom) which are combinations of bit-wise and
arithmetic operators like bit-wise OR, AND, multiplication, subtraction,
shifts and other C operators.

\begin{figure*}[htbp]
\scriptsize
\begin{tabular}{l|l|l}
\hline
Bit-select & Part-select (System Verilog) & Concatenation \\
\hline
\begin{lstlisting}[mathescape=true,language=Verilog]
wire [7:0] in1,in2;
reg [7:0] out1,out2;
out1[7:5] = in1[4:2];
out2[6] = in2[4];
\end{lstlisting}
&
\begin{lstlisting}[mathescape=true,language=Verilog]
reg [31:0] in, out;
for(i=0;i<=3;i++) begin
out[8*i +: 8]=in[8*i +: 8];
end
\end{lstlisting}
&
\begin{lstlisting}[mathescape=true,language=Verilog]
wire [7:0] in1, in2;
reg [9:0] out;
out = {in2[5:2],in1[6:1]};
\end{lstlisting}
\\
\hline
\begin{lstlisting}[mathescape=true,language=C]
unsigned char in1,in2;
struct smain { 
 unsigned char out1,out2; } sm;
sm.out1 = sm.out1 & 0x1f | 
(((in1 & 0x1c)>>2)<<5);
sm.out2 = (sm.out2 & 0xbf)| 
(((in2 & 0x10)>>4)<<6); 
\end{lstlisting}
&
\begin{lstlisting}[mathescape=true,language=C]
struct smain {
 unsigned int in,out; } sm;
for(i=0;i<=3;i++) {
 x=8*i+(8-1); y=8*i;
 sm.out=(sm.out&!(2^31-2^y))
 |(sm.in&(2^31-2^y)); }
\end{lstlisting}
&
\begin{lstlisting}[mathescape=true,language=C]
unsigned char in1,in2;
struct smain { 
 unsigned char out; } sm;
sm.out = (((in2 >> 2)
 & 0xF) << 6)|
 ((in1 >> 1) & 0x3F);
\end{lstlisting}
\\
\hline
\end{tabular}
\caption{Handling Bit-select, part-select from vectors and concatenation}
\label{figure:bit}
\end{figure*}

%=======================================================================================
\section{Monolithic and Path-based Symbolic Execution} 
%=======================================================================================
Figure~\ref{figure:simulation} gives the path constraints generated 
by path-based and BMC based tools. Given a program fragment on the 
left shown in column~1, the path constraints corresponding to three paths 
in the program is shown in column~[2--4]. Note that all paths in this 
program are feasible. The monolithic path constraint generated by BMC 
is shown in column~5. BMC-based tools \emph{always} merges---generating 
only a \emph{single} bit-vector formula $C$ for a given unwinding bound $k$.  Note that 
this formula is linear in the size of the program and linear in $k$ 
even if there is an exponential number of paths in the program.  
For the constriant in column~5, the symbolic values of variables 
are computed as expressions over the initial values of variables 
$m$ and $t$, whereas the branching in the program yields expressions with 
the $\mathit{ite}$ operator.  

\begin{figure}[t]
\scriptsize
\begin{tabular}{l|l|l|l|l}
\hline
Program & Path & Path & Path & Monolithic \\
        & Constraint 1 & Constraint 2 & Constraint 3 & Constraint\\
\hline
\begin{lstlisting}[mathescape=true,language=C]
void top(){
 if(reset) {
  m = 0;
  t = 0;
 }
 else {
  if(c > d)
   m = c+d;
  else
   t = (c & 3)<<d;
 }
}
\end{lstlisting}
&
\begin{minipage}{1.5cm}
$\begin{array}[t]{@{}l}
C_1 \; \equiv \\
\;\;\mathit{\mathit{reset}}_1 \neq 0\; \land \\
\;\; m_2 = 0\;\land \\
\;\; t_2 = 0
\end{array}$
\end{minipage}
&
\begin{minipage}{1.5cm}
$\begin{array}[t]{@{}l}
C_2 \; \equiv \\
\;\;\mathit{\mathit{reset}}_1=0\; \land \\
\;\;d_1 \ngeq c_1\; \land \\
\;\;m_3 = c_1 + d_1
\end{array}$
\end{minipage}
&
\begin{minipage}{1.5cm}
$\begin{array}[t]{@{}l}
C_3\; \equiv \\
\;\;\mathit{\mathit{reset}}_1 = 0\; \land \\
\;\;d_1 \ge c_1\; \land \\
\;\;t_3 = (c_1\&3) \\
          <\!\!<d_1
\end{array}$
\end{minipage}
&
\begin{minipage}{5cm}
$\begin{array}{l@{\,\,}c@{\,\,}l}
C &\iff& ((\mathit{\mathit{guard}}_1 =  \neg(\mathit{\mathit{reset}}_1 = 0)) \land \\
  &    & (m_2 = 0) \land (t_2 = 0) \land \\
  &    & (m_3 = m_1) \land (t_3 = t_1) \land \\
  &    & (\mathit{guard}_2 = \neg(d_1 >= c_1)) \land \\
  &    & (m_4 = c_1 + d_1) \land (m_5 = t_3) \land \\
  &    & (t_4 = (c_1 \& 3) <\!\!< d_1) \land \\
  &    & (x_6 = \mathit{ite}(\mathit{\mathit{guard}}_2, m_4, m_5)) \land \\
  &    & (t_5 = \mathit{ite}(\mathit{\mathit{guard}}_2, t_3, t_4)) \land \\
  &    & (m_7 = \mathit{ite}(\mathit{\mathit{guard}}_1, 0, m_6)) \land \\
  &    & (t_6 = \mathit{ite}(\mathit{\mathit{guard}}_1, 0, t_5)))
\end{array}$
\end{minipage}
\\
\hline 
\end{tabular} 
\caption{Path-based and monolithic symbolic execution}
\label{figure:simulation}
\end{figure}

%=======================================================================================
\section{Firmware Model in Hardware/Software Co-verification} 
%=======================================================================================
Figure~\ref{firmware} shows a fragment of the firmware model for the UART IP. 
The firmware implements linux style inb() and outb() functions to communicate 
with the hardware ports. The $wb$ class of functions communicate with the 
wishbone bus interface. The $set\_inputs()$ and the $next\_timeframe()$
functions are the primitives for \textsc{HW-CBMC} that direct the tool 
to set the inputs to the hardware signals and advance the clock signal 
respectively. In the monolithic software netlist model, this is implemented 
by actually invoking the top level function in the software netlist model. 
The top level function in software netlist corresponds to the top module 
of the UART IP core. 

The firmware begins by resetting the UART IP which is followed by a $wb\_idle()$  
function. Then, the actual operation starts by setting the appropriate values to
the memory mapped registers which is propagated to the hardware modules.  
The firmware here sets the UART in loopback mode with interrupt enabled. We 
verify properites over the hardware firmware interactions. In particular, we 
verify whether the transmitted data is same as the received data in the loopback
mode. This is done by putting an assertion in the firmware model that checks the 
data from the transmitter and the receiver module. 
 
\begin{figure*}
\scriptsize
\begin{tabular}{l|l}
\hline
Wishbone Interface & Firmware \\
\hline
\begin{lstlisting}[mathescape=true,language=C]
typedef unsigned char u8;
unsigned char inb 
 (unsigned long port) {
  return wb_read(port);
}
void outb (u8 value, 
 unsigned long port) {
  wb_write(port, value);
}
void wb_reset(void) {
 rtfSimpleUart.rst_i = 1;
 set_inputs();
 next_timeframe();
 rtfSimpleUart.rst_i = 0;
 rtfSimpleUart.stb_i = 0; 
 rtfSimpleUart.cyc_i = 0;
}
void wb_idle() {
 set_inputs();
 next_timeframe();
}
void wb_write(_u32 addr, 
             _u8 b) {
 rtfSimpleUart.adr_i = addr;
 rtfSimpleUart.dat_i = b;
 rtfSimpleUart.we_i = 1;
 rtfSimpleUart.cyc_i = 1;
 rtfSimpleUart.stb_i = 1;
 set_inputs();
 next_timeframe();
 rtfSimpleUart.we_i = 0;
 rtfSimpleUart.cyc_i = 0;
 rtfSimpleUart.stb_i = 0;
}
\end{lstlisting}
&
\begin{lstlisting}[mathescape=true,language=C]
int main() {
wb_reset();
wb_idle();
// Configure the uart
outb (0x13, UART_MC);  
outb (0x80, UART_CM3);
outb (0x00, UART_CM2);
outb (0x00, UART_CM1);
outb (0x00, UART_CR);  
outb (0x03, UART_IE); 
char tx_b[] = "Hello world";
_u8 istatus = 0;
char rx_b[100];
int i=0,c=0,d=0;
for (i=0; i<1990; i++){
if (rtfSimpleUart.irq_o){
 istatus=inb(UART_IS)&0x0c;
 if(istatus==0x0c){
 //it was a tx_empty interrupt
 outb(*(tx_b+c),UART_TR);
 c++;
 }
 else{//istatus==0x04
 //it was an rx_data interrupt
  rx_b[d] = inb(UART_TR);
  d++;
 }
}else {
 // no interrupt. 
 wb_idle();
 wb_idle();
 }
}
for(i=0; i<=10; i++)
 assert(rx_b[i] == tx_b[i]);
}
\end{lstlisting}
\\
\hline
\end{tabular}
\caption{Firmware model for UART IP}
\label{firmware} 
\end{figure*}

\newpage
%=======================================================================================
\section{\verifox: Tool Flow} 
%=======================================================================================
Figure~\ref{verifox} shows the overall tool flow for \verifox. Given a 
hardware desing in Verilog RTL and a property in System Verilog Assertion
language (SVA), the tool \emph{v2c} automatically generate the software netlist 
model in C following the synthesis semantics. Our experimental result shows that 
the proposed tool flow can be used for hardware property verification as well as 
co-verification in the peresence of a firmware. A monolithic model is generated in
C along with the firmware or a user-specified assumption which specify the 
partition constraint for state-space decomposition. The tool perform
property-driven slicing on the monolithic C program. The sliced program is then
passed to the symbolic execution engine. This engine explores the input 
sliced program in a depth-first manner with aggressive path pruning strategy. 
The generated path-constraints are encoded incrementally and passed to the
underlying solver only if it is feasible. \verifox either shows that the program 
is correct with respect to the given assertions or returns a counterexample
trace violating the property. The command line option to run verifox is shown
below:
\begin{lstlisting}[basicstyle=\scriptsize]
verifox-pi <C-file-name> // partial incremental mode with SAT
verifox-fi <C-file-name> // full incremental mode with SAT
\end{lstlisting}
\begin{figure*}

\tikzstyle{rblock}=[rounded corners,draw=black]
\tikzstyle{block}=[draw=black]
\centering
\begin{tikzpicture}

\node (v2c) [rblock] {\scs{\emph{v2c}}};
\node (snl) [block,below of=v2c] {\scs{Software-netlist}};
\draw[->] (v2c) -- (snl);

\node (HD) [above left=.3cm and .3cm of v2c] {\scs{\parbox{8em}{Hardware Design \\ (in Verilog)}}};
\draw[->] (HD) -- (v2c);

\node (prop) [above right=.3cm and .3cm of v2c] {\scs{\parbox{8em}{Property \\ (in SVA)}}};
\draw[->] (prop) -- (v2c);

\node (cmm) [block,below of=snl] {\scs{\parbox{9em}{Composite Monolithic Model}}};
\draw[->] (snl) -- (cmm);

\node (dcmm) [left=1cm of cmm] {};
\node (fw) [above=.1cm of dcmm  ] {\scs{Firmware}};
\node (as) [below=.1cm of dcmm] {\scs{Assumptions}};
\draw[->] (fw) -- (cmm);
\draw[->] (as) -- (cmm);

\node (pds) [block,below of=cmm] {\scs{\parbox{8em}{Property-driven slicing}}};
\draw[->] (cmm) -- (pds);

\node (tp) [block,below=.8cm of pds] {\scs{Paths Exploration}};
\node (iss) [block,below right=.5cm  and .05cm of tp.east] {\scs{\parbox{6em}{Incremental SAT solving}}};
\node (sat) [rblock,below=1.5cm of tp] {\scs{SAT solver}};
\node (ipp) [block,left=2cm of iss] {\scs{\parbox{6em}{Infeasible path pruning}}};

\draw [<->] (tp) -- (iss);
\draw [<->] (tp) -- (ipp);
\draw [<->] (sat) -- (iss);
\draw [<->] (sat) -- (ipp);

\node (vfbox) [rblock,fit={(tp) (iss) (sat) (ipp)}] {};
\draw[->] (pds) -- (vfbox);

\node (verifox) [right=.2cm of tp] {\scs{{\bf \verifox}}};

\node (safe) [above right=.2cm and .2cm of vfbox.east] {\scs{Verification Successful}};
\node (unsafe) [below right=.2cm and .2cm of vfbox.east] {\scs{\parbox{8em}{Verification Failed (Counterexample)}}};

\draw[->] (vfbox.9) -- (safe);
\draw[->] (vfbox.-12) -- (unsafe);

\end{tikzpicture}
\caption{\verifox tool flow \label{verifox}}
\end{figure*}
